# Supplementary material for: A spatially extended model to assess the role of landscape structure on the pollination service of Apis mellifera
Source: arXiv:1907.08481 ancillary file (2020-07-06)
Supplement: Supplementary file 1 [file apis-09_sup.pdf]

# A spatially extended model to assess the role of landscape structure on the pollination service of Apis mellifera

Julien Joseph[a,d,*], Fernanda Santibáñez[b,c], María Fabiana Laguna[d], Guillermo Abramson[d,e], Marcelo N. Kuperman[d,e], Lucas A. Garibaldi[b,c]

[a]École Normale Supérieure de Lyon, Université Claude Bernard Lyon I, Université de Lyon, 69342 Lyon Cedex 07, France.
[b]Universidad Nacional de Río Negro. Instituto de Investigaciones en Recursos Naturales, Agroecología y Desarrollo Rural. San Carlos de Bariloche, Río Negro, Argentina.
[c]Consejo Nacional de Investigaciones Científicas y Técnicas. Instituto de Investigaciones en Recursos Naturales, Agroecología y Desarrollo Rural. San Carlos de Bariloche, Río Negro, Argentina.
[d]Centro Atómico Bariloche (CNEA) and CONICET, R8402AGP Bariloche, Argentina.
[e]Instituto Balseiro, Universidad Nacional de Cuyo, R8402AGP Bariloche, Argentina.

Supplementary material

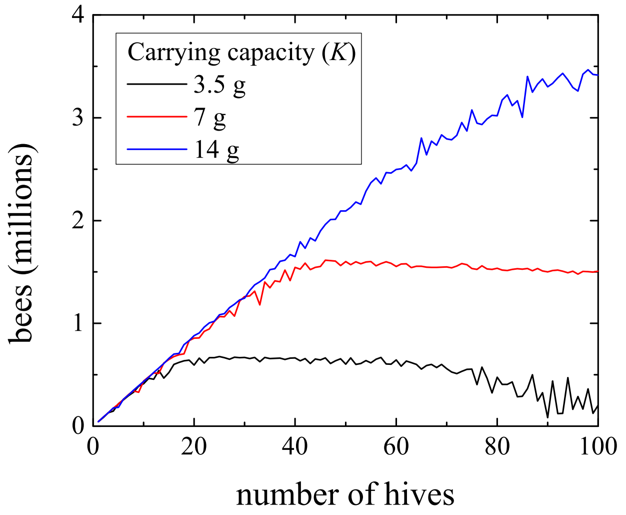


Figure S.1: The effect of local competition on the number of bees. This plot complements Fig. 1, corresponding to a synthetic map with 4% natural resource and edge density 0.19. The crop blooming period is from day 20 to day 55, with day 0 the first day of spring. The model ran 2 years, and we took the values for the second year.

*Corresponding author
Email addresses: julien.joseph@ens-lyon.fr (Julien Joseph), fsantibanez@unrn.edu.ar (Fernanda Santibáñez), lagunaf@cab.cnea.gov.ar (María Fabiana Laguna), abramson@cab.cnea.gov.ar (Guillermo Abramson), kuperman@cab.cnea.gov.ar (Marcelo N. Kuperman), lgaribaldi@unrn.edu.ar (Lucas A. Garibaldi)

Submitted to Ecological modelling

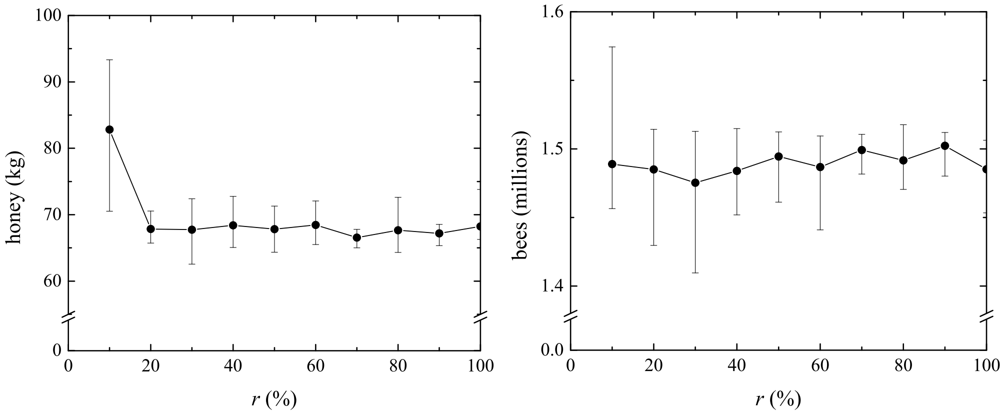


Figure S.2: Average number of honey and bees (with minimum and maximum shown as error bars). The crop blooming period is from day 20 to day 55, with day 0 the first day of spring. The model ran 2 years with 100 hives placed at random on the border of the natural habitat, and we took the values for the second year. These plots complement Fig. 2.

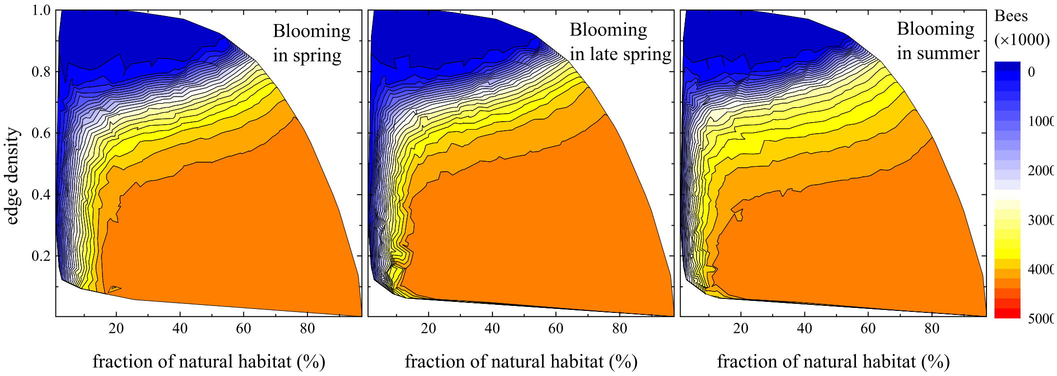


Figure S.3: Mean annual number of bees as a function of the fraction of natural habitat and the edge density. The color scale shows the mean annual total number of visits. Left: crop blooming period from day 22 to day 55. Middle: crop blooming period from day 80 to day 115. Right: crop blooming period from day 130 to day 165. Day 0 is the first day of spring. We used 1000 maps for each of these analyses.

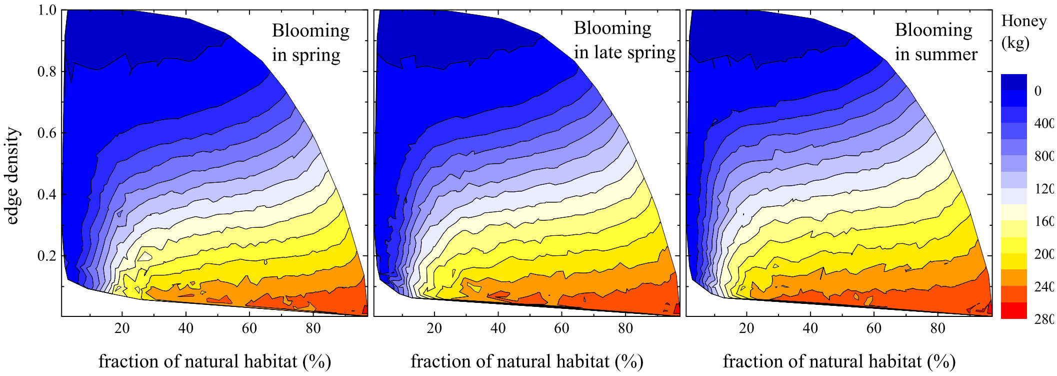


Figure S.4: Mean annual honey production as a function of the fraction of natural habitat and the edge density. The color scale shows the mean annual total number of visits. Left: crop blooming period from day 22 to day 55. Middle: crop blooming period from day 80 to day 115. Right: crop blooming period from day 130 to day 165. Day 0 is the first day of spring. We used 1000 maps for each of these analyses.

Table S.1: Sensitivity analysis of the model with one single hive placed in a map with only natural habitat. Each default value of the parameter was either divided by 2 or multiplied by 2, and the percentage of the difference compared to the default values are shown. Gray cells indicate the death of the colony. A hyphen indicates no significant variation (less than 1%).

Most of these parameters are from the hive dynamic model of [1]: $\alpha_{min} = 0.25$ (rate that hive bees become foragers), $\alpha_{max} = 0.25$ (controls how low food stores affect the transition to foraging), $b = 500$ and $v = 5000$ (parameters in the phenomenological survival rate of brood), $\sigma = 1.3$ (strength of social inhibition on forager population), $L = 2000$ (laying rate of the queen), $\phi = 1/9$ (adults' emerging rate from pupation), $\tau = 21$ (pupation time), $m = 0.06$ (foragers' death rate), $\gamma_A = 0.007$ (consumption of stored food by adults), $\gamma_B = 0.018$ (consumption of stored food by brood), $c = 0.09$ (average food collected per forager per day, in grams).

Besides, as described in the main text: $k = 200$ (foraging squad size), $N_{trips} = 19$ (trips per forager per day), $N_{flower,trip} = 75$ (flowers visited in one forager's trip), $r_f = 3$ (maximum foraging distance, in km).

[1] Khoury et al., Modelling food and population dynamics in honey bee colonies. PLOS ONE 8:e59084 (2013).

| | ×2 | | | ÷2 | | |
|---|---|---|---|---|---|---|
| Parameter | Number of bees | Quantity of honey | Number of visits | Number of bees | Quantity of honey | Number of visits |
| $\alpha_{min}$ | | | | +72.9% | −90.0% | −9.2% |
| $\alpha_{max}$ | - | −3.3% | −3.5% | - | - | - |
| $b$ | −1.3% | −8.0% | −7.4% | - | +3.9% | +4.3% |
| $\sigma$ | +65.3% | −85.5% | −10.9% | −43.4% | +9.9% | −21.7% |
| $L$ | +117.4% | +137.9% | +134.7% | −61.6% | −70.2% | −69.3% |
| $v$ | −19.4% | −31.6% | −29.3% | +8.5% | +17.6% | +14.8% |
| $\phi$ | - | +73.2% | +8.4% | | | |
| $\tau$ | −4.8% | −34.1% | −22.0% | - | +16.5% | +9.7% |
| $m$ | | | | +86.4% | +247.3% | +110.0% |
| $\gamma_B$ | −78.5% | −98.3% | −77.9% | - | +63.8% | +2.6% |
| $\gamma_A$ | −18.7% | −93.3% | −26.7% | - | +58.7% | +2.3% |
| $c$ | - | +349.6% | +5.0% | | | |
| $k$ | - | - | - | - | - | - |
| $N_{trips}$ | - | - | +100.0% | - | - | −50.0% |
| $N_{flower,trip}$ | - | - | +100.0% | - | - | −50.0% |
| $r_f$ | - | +22.5% | +13.9% | - | −8.0% | - |
